# Supplementary material for: Dynamics of Majority Rule on Hypergraphs
Source: arXiv:2101.03632 source file (2021-01-10)
Supplement: Supplementary file 1 [file appendix1.tex]

\chapter{The Redirection Algorithm}\label{Redirection}
In this Appendix we describe the way in which the redirection algorithm is used to construct scale-free networks \cite{li2005towards}. This complements the analysis presented in Section \ref{scalefree}. We use \cite[Chapter 14]{krapivsky2010kinetic} as the primary reference for our discussion, though additional calculations are provided where necessary. The redirection algorithm works as follows:
\begin{enumerate}
    \item Pick a pre-existing node \textbf{x} from the network uniformly at random.
    \item Introduce a new node \textbf{n}. With probability $1-r$, the new node \textbf{n} attaches to node \textbf{x}, where $r\in\left[0,1\right]$.
    \item With probability $r$, \textbf{n} attaches to the ancestor node \textbf{y} of node \textbf{x}. The ancestor node \textbf{y} is the node to which \textbf{x} attached upon its introduction to the network.
\end{enumerate}
In order to initialise the algorithm we start with two connected nodes, each of which is the ancestor of the other. In general, the evolution of a degree distribution where network growth is dictated by an attachment rate $A_{k}$ is given by the following equation:
 \begin{equation}\label{attachmentME}
     \frac{dN_{k}}{dN} = \frac{A_{k-1}N_{k-1}-A_{k}N_{k}}{A}+\delta_{k1},
 \end{equation}
 where $N_{k}$ is the number of nodes in the network of degree $k$, $N$ is the total number of nodes in the network, and $A = \sum_{j\geq 1}A_{j}N_{j}$. Equation (\ref{attachmentME}) may be explained as follows: the first term on the right hand side accounts for an increase in $N_{k}$ when a new node attaches itself to a pre-existing node of degree $k-1$. The second term on the right hand side accounts for the decrease in $N_{k}$ when a new node attaches itself to a pre-existing node of degree $k$. Finally the Kronecker delta function $\delta_{k1}$ accounts for the introduction of a new node of degree $1$.
Under the redirection algorithm, the degree distribution of a network evolves according to the following equation:
 \begin{equation}
     \frac{dN_{k}}{dN} = \frac{1-r}{N}\left[N_{k-1}-N_{k}\right]+\delta_{k1}+\frac{r}{N}\left[\left(k-2\right)N_{k-1}-\left(k-1\right)N_{k}\right]. \label{redirectionRate}
 \end{equation}
 In the event that $r=0$, equation (\ref{redirectionRate}) describes a system whereby at each update, a new node is introduced that attaches to a pre-existing node in the network chosen uniformly at random. This describes the evolution of random recursive trees \cite[Section 14.3]{krapivsky2010kinetic}. For the redirection algorithm to be of any use we therefore require $r>0$, which we will assume from now on. Under this assumption, equation (\ref{redirectionRate}) may be rearranged to give
 \begin{equation}
     \frac{dN_{k}}{dN} = \frac{r}{N}\left[\left(k-1+\left(\frac{1}{r}-2\right)\right)N_{k-1}-\left(k+\left(\frac{1}{r}-2\right)\right)N_{k}\right]+\delta_{k1}. \label{redirectionrearranged}
 \end{equation}
 Comparing equations (\ref{attachmentME}) and (\ref{redirectionrearranged}) we observe that the redirection algorithm corresponds to an attachment rate $A_{k} = k+1/r-2$ which is a linear function of $k$. Therefore the redirection algorithm inadvertently gives rise to linear preferential attachment, which can be used to construct scale-free networks at relatively low computational cost. \newline
 
 \noindent We shall now derive the degree distribution of a network whose growth is governed by the redirection algorithm. To do so we first consider the moments of the degree distribution $M_{\alpha}\left(N\right) = \sum_{j}j^{\alpha}N_{j}$. As the network grows, the evolution of the zeroth and first moments are straightforward to calculate:
 \begin{align}
     &\frac{dM_{0}}{dN} = \frac{1}{N}\sum_{j\geq 1}N_{j} = \frac{N}{N} = 1, \label{M0} \\
     &\frac{dM_{1}}{dN} = \sum_{j\geq 1}j\frac{dN_{j}}{dN} = \sum_{j}j\left(\frac{A_{j-1}N_{j-1}-A_{j}N_{j}}{A} + \delta_{j1}\right) = \frac{1}{A}\sum_{j\geq 1}A_{j}N_{j} + 1 = 2. \label{M1}
 \end{align}
 This shows that the zeroth and first moments scale linearly with $N$. Therefore if we choose the attachment rate to be $A_{k}=k^{\beta}$ with $\beta\in\left[0,1\right]$, the total rate $A = \sum_{j}j^{\beta}N_{j}$ is bounded below by the zeroth moment and above by the first moment. This implies that the total rate in this instance grows linearly with $N$. Therefore we make the asymptotic approximation $A\approx\mu N$ where $\mu$ is a scalar that varies smoothly between $1$ and $2$ as $\beta$ varies between $0$ and $1$. Using this approximation, it is straightforward to solve equation (\ref{attachmentME}) for $k\geq 1$ using integrating factors of the form $N^{A_{k}/\mu}$:
 \begin{align}
     &\frac{dN_{1}}{dN} =-\frac{A_{1}N_{1}}{A}+1 \Rightarrow N_{1} = \frac{\mu}{A_{1}}\left(1+\frac{\mu}{A_{1}}\right)^{-1}N, \label{dN1}\\
     &\frac{dN_{2}}{dN} = \frac{A_{1}N_{1}-A_{2}N_{2}}{A} \Rightarrow N_{2} = \frac{\mu}{A_{2}}\left(1+\frac{\mu}{A_{1}}\right)^{-1}\left(1+\frac{\mu}{A_{2}}\right)^{-1}N. \label{dN2}
 \end{align}
 From solving the first few equations it is clear that $N_{k}$ is proportional to $N$ for all $k\geq 1$. Making the substitution $n_{k} = N_{k}/N$ transforms equation (\ref{attachmentME}), resulting in the following system:
 \begin{align}
     n_{1} &= -\frac{A_{1}n_{1}}{\mu}+1\quad\text{for}\quad k=1, \nonumber \\
     n_{k} &= \frac{A_{k-1}n_{k-1}-A_{k}n_{k}}{\mu}\quad\text{for}\quad k>1. \label{nksystem}
 \end{align}
 Rescaling the rate equation in this way allows for the more convenient study of the degree distribution. From equations (\ref{dN1}) and (\ref{dN2}) it is straightforward to see that the general solution of system (\ref{nksystem}) is given by
 \begin{equation}\label{nkequation}
     n_{k} = \frac{\mu}{A_{k}}\prod_{1\leq j\leq k}\left(1+\frac{\mu}{A_{j}}\right)^{-1}.
 \end{equation}
 To prove this by induction we take equation (\ref{dN1}) as the base case. Now assume that for some $k>1$, equation (\ref{nkequation}) holds. Then for $n_{k+1}$ we have
 \begin{align*}
     &n_{k+1}\left(1+\frac{A_{k+1}}{\mu}\right) = \prod_{1\leq j\leq k}\left(1+\frac{\mu}{A_{j}}\right)^{-1} \Rightarrow n_{k+1} = \left(1+\frac{A_{k+1}}{\mu}\right)^{-1}\prod_{1\leq j\leq k}\left(1+\frac{\mu}{A_{j}}\right)^{-1} \\
     &=\left(\frac{A_{k+1}}{\mu}\right)^{-1}\left(1+\frac{\mu}{A_{k+1}}\right)^{-1}\prod_{1\leq j\leq k}\left(1+\frac{\mu}{A_{j}}\right)^{-1} = \frac{\mu}{A_{k+1}}\prod_{1\leq j\leq k+1}\left(1+\frac{\mu}{A_{j}}\right)^{-1}.
 \end{align*}
 This completes the inductive proof of equation (\ref{nkequation}). \newline
 
 \noindent Using equation (\ref{nkequation}) we can derive the degree distribution of networks constructed via the redirection algorithm. Consider a shifted linear attachment rate of the form $A_{k} = k + \gamma$ where $\gamma\in\mathbb{R}$. Then we can express $A$ as 
 \begin{equation*}
     A = \sum_{j}N_{j}A_{j} = \sum_{j}N_{j}\left(j+\gamma\right) = \gamma M_{0}+M_{1} = \left(2+\gamma\right)N \approx \mu N
 \end{equation*}
 where in this case the amplitude $\mu=2+\gamma$. Substituting this expression for $\mu$ into equation (\ref{nkequation}) yields:
 \begin{align*}
     n_{k}&=\frac{\mu}{A_{k}}\prod_{1\leq j\leq k}\left(1+\frac{\mu}{A_{j
    }}\right)^{-1} = \frac{2+\gamma}{j+\gamma}\prod_{1\leq j\leq k}\left(1+\frac{2+\gamma}{k+\gamma}\right)^{-1} = \frac{2+\gamma}{k+\gamma}\prod_{1\leq j\leq k}\left(\frac{j+2+2\gamma}{j+\gamma}\right)^{-1} \\
    &=\left(2+\gamma\right)\frac{\Gamma\left(k+\gamma\right)\Gamma\left(2\gamma+3\right)}{\Gamma\left(1+\gamma\right)\Gamma\left(2\gamma+k+3\right)},
 \end{align*}
 which is of the form of a discrete power law. It is more informative to consider the asymptotic degree distribution which may be derived as follows:
 \begin{align*}
     n_{k}&=\frac{\mu}{A_{k}}\prod_{1\leq j\leq k}\left(1+\frac{\mu}{A_{j
    }}\right)^{-1} = \frac{\mu}{k+\gamma}\exp\left(-\sum_{j=1}^{k}\ln\left(1+\frac{\mu}{j+\gamma}\right)\right)^{-1} \\
    &\sim \frac{\mu}{k+\gamma}\exp\left(-\int_{1}^{k}\ln\left(1+\frac{\mu}{j+\gamma}\right)\textit{dj}\right) \\ &\approx \frac{\mu}{k+\gamma}\exp\left(-\int_{1}^{k}\left(\frac{\mu}{j+\gamma}+O\left(\left(j+\gamma\right)^{-2}\right)\right)\textit{dj}\right) \\
    &\approx \frac{\mu}{k+\gamma}\exp\left(-\int_{1}^{k}\frac{\mu}{j+\gamma}\textit{dj}\right) = \mu\left(1+\gamma\right)^{\mu}\left(k+\gamma\right)^{-\mu-1} \sim \left(k+\gamma\right)^{-\mu-1} \\
    &= k^{-\mu-1}\left(1+\frac{\gamma}{k}\right)^{-\mu-1}\approx k^{-\mu-1}\sim k^{-3-\gamma}.
 \end{align*}
 The redirection algorithm is a particular instance of linear preferential attachment with $\gamma = 1/r -2$. Therefore redirection can be used to generation degree distributions of the form
 \begin{equation}\label{nkrdistribution}
     n_{k}\sim k^{-1-1/r}.
 \end{equation}
 In this way, we can vary the selection parameter $r$ to construct networks with distribution $k^{-\chi}$ for any $\chi>2$. This equips us with the structural foundations necessary to study MR dynamics on scale-free networks.
